# Supplementary material for: Direct Distillation between Different Domains
Source: arXiv:2401.06826 source file (2024-01-12)
Supplement: Supplementary file 1 [file X_suppl.tex]

\clearpage
\setcounter{page}{1}
\maketitlesupplementary
In this section, we provide supplementary materials for our proposed Direct Distillation between Different Domains (4Ds), including: 1) The details of traditional knowledge distillation (in Section~\ref{sec:tkd}); 2) The pseudo-codes for key components in our proposed 4Ds (in Section~\ref{sec:psc}); 3) The explanation of feature mapping operation (in Section~\ref{sec:fmo}); 4) Structural analysis of the knowledge adapter (in Section~\ref{sec:saka}); 5) Parameter sensitivity analysis of hyper-parameters in our proposed 4Ds (in Section~\ref{sec:ps}); 6) Details of various weighting strategies for domain-invariant features (in Section~\ref{sec:ws}).
\subsection{Traditional Knowledge Distillation}
\label{sec:tkd}
Vanilla Knowledge Distillation (KD) methods~\cite{hinton2015distilling,chen2022knowledge} train a compact student network $\mathcal{N}_{S}$ by learning from a powerful pre-trained teacher network $\mathcal{N}_{T}$. Formally, the training dataset for both $\mathcal{N}_{T}$ and $\mathcal{N}_{S}$ is denoted as $\mathcal{D}=\left\{\left(\mathbf{x}_i, y_i\right)\right\}_{i=1}^{|\mathcal{D}|}$. Given an input example $\mathbf{x}_{i} \in \mathcal{D}$, vanilla KD is achieved by minimizing the following loss function:
\begin{equation}
\mathcal{L}_{\mathrm{kd}}\left(\mathcal{N}_S\right)=\frac{1}{|\mathcal{D}|} \sum_{i=1}^{|\mathcal{D}|}\left[\mathcal{H}_{\mathrm{ce}}\left(\mathcal{N}_S\left(\mathbf{x}_i\right), y_i\right)+\lambda \mathcal{H}_{\mathrm{kt}}\left(\mathbf{f}_i^S, \mathbf{f}_i^T\right)\right],
\end{equation}
where $\mathcal{H}_{\mathrm{ce}}$ is the \textbf{c}ross-\textbf{e}ntropy loss function, and it promotes $\mathcal{N}_{S}$ to predict results as consistent as the ground-truth labels; $\mathcal{H}_{\mathrm{kt}}$ stands for the \textbf{k}nowledge \textbf{t}ransfer loss function, which encourages $\mathcal{N}_{S}$ to mimic the knowledge $\mathbf{f}_i^T$ acquired by $\mathcal{N}_{T}$, and here the notations with superscripts ``$T$'' and ``$S$'' denote that they are related to $\mathcal{N}_{T}$ and $\mathcal{N}_{S}$, respectively; $\lambda>0$ is the trade-off parameter to balance $\mathcal{H}_{\mathrm{ce}}$ and $\mathcal{H}_{\mathrm{kt}}$.

Traditional KD methods, however, may encounter difficulties when training the student network in a new target domain that is significantly different from the teacher's source domain, as discussed in Section~\ref{sec:intro}. Therefore, to address this issue, we propose 4Ds, a novel one-stage framework for distilling a student network in the new target domain.
\subsection{Pseudo-Code}
\label{sec:psc}
In this subsection, we provide the pseudo-codes for the adapter and fusion-activation mechanism. Alg.~\ref{alg_pyad} shows the pseudo-code of the adapter, the input feature is first adapted by two 1$\times$1 convolutional layers with Batch Normalization (BN) layer and ReLU activation function on the target data. Then, the adapted feature and input feature are converted as frequency features by the Fourier transform and decomposed into amplitude and phase components. Subsequently, the amplitude is refurbished by composing the amplitudes decomposed from the adapted feature and original input feature with the learnable weights. In the end, the refurbished amplitude and original phase are composed as frequency feature and transferred to spatial feature via the inverse Fourier transform.

The pseudo-code of the fusion-activation mechanism is depicted in Alg.~\ref{alg_pyfa}. Firstly, the features produced by various blocks of the network are scaled to the same size of $H\times W$ and concatenated together. Then, the concatenated features are squeezed to the size of $1\times 1$ and mapped as the attention weights. Finally, the concatenated features are activated by the attention weights.
\begin{algorithm}[t]
	\caption{Pseudo-code of Adapter in PyTorch-like Style.}
	% \algcomment{\fontsize{7.2pt}{0em}\selectfont \texttt{bmm}: batch matrix multiplication; \texttt{mm}: matrix multiplication; \texttt{cat}: concatenation.
	% %\vspace{-1.em}
	% }
	\definecolor{codeblue}{rgb}{0.25,0.5,0.5}
	\lstset{
		backgroundcolor=\color{white},
		basicstyle=\fontsize{7.2pt}{7.2pt}\ttfamily\selectfont,
		columns=fullflexible,
		breaklines=true,
		captionpos=b,
		commentstyle=\fontsize{7.2pt}{7.2pt}\color{codeblue},
		keywordstyle=\fontsize{7.2pt}{7.2pt},
		%  frame=tb,
	}
	
	% # atan2, cos, sin: arctangent, cosine, sine function
	% # complex: transfer function tensor view to complex number
	\begin{lstlisting}[language=python]
# conv: 1x1 convolutional layer
# decompose: frequency feature to amplitude and phase
# compose: amplitude and phase to frequency feature
# weights: learnable parameters, t: temperatures
def adapter(f):
    weights_soft = softmax(weights/t, dim=0) 
    f_ad = bn(conv(relu(bn(conv(f))))) # adapt f
    F = FT(f) # FT: fourier transform
    F_ad = FT(f_ad)
    a, p = decompose(F) # a: amplitude, p: phase
    a_ad, p_ad = decompose(F_ad)
    f_ift = IFT(compose(a_ad * weights_soft[0] + a * weights_soft[1], p)) # IFT: inverse FT
    return f_ift
	\end{lstlisting}
	\label{alg_pyad}
\end{algorithm}
\begin{algorithm}[t]
\caption{Pseudo-code of Fusion-Activation Mechanism in PyTorch-like Style.}
% \algcomment{\fontsize{7.2pt}{0em}\selectfont \texttt{bmm}: batch matrix multiplication; \texttt{mm}: matrix multiplication; \texttt{cat}: concatenation.
% %\vspace{-1.em}
% }
\definecolor{codeblue}{rgb}{0.25,0.5,0.5}
\lstset{
	backgroundcolor=\color{white},
	basicstyle=\fontsize{7.2pt}{7.2pt}\ttfamily\selectfont,
	columns=fullflexible,
	breaklines=true,
	captionpos=b,
	commentstyle=\fontsize{7.2pt}{7.2pt}\color{codeblue},
	keywordstyle=\fontsize{7.2pt}{7.2pt},
	%  frame=tb,
}

% # atan2, cos, sin: arctangent, cosine, sine function
% # complex: transfer function tensor view to complex number
\begin{lstlisting}[language=python]
# fs: a set of features
# B: batchsize
def fusion-activation(fs):
    _, _, H, W = fs[3].size() # H: height, W: width
    f0 = avg_pool(fs[0], (H, W)) # resize fs[0] to H x W
    f1 = avg_pool(fs[1], (H, W))
    f2 = avg_pool(fs[2], (H, W))
    f3 = fs[3]
    f = cat((f0, f1, f2, f3), dim=1) # fuse f0, f1, f2, f3 as f: B x M x H x W
    z = avg_pool(f, (1, 1)) # squeeze f to 1 x 1
    s = sigmoid(fc(relu(fc(z)))) # map z as attention weights
    f_act = f * s.expand_as(f) # activate f
    return f_act
\end{lstlisting}
\label{alg_pyfa}
\end{algorithm}
\subsection{Feature Mapping Operation}
\label{sec:fmo}
The domain-invariant transfer in our method may be hindered by the feature dimension mismatched between the teacher and student networks. Therefore, we address this issue by employing a feature mapping operation to align the feature dimensions of the teacher and student networks. 

Given the fused features $\mathcal{P}^{T}_{\text{fuse}} \in \mathbb{R}^{C_{T} \times H_{T} \times W_{T}}$ and $\mathcal{P}^{S}_{\text{fuse}}\in \mathbb{R}^{C_{S} \times H_{S} \times W_{S}}$ of the teacher and student networks, respectively. Here, $C$, $H$, and $W$ denote the number of channels, height, and width of the corresponding feature, respectively. When the feature map dimensions of the teacher network are larger than those of the student network (\emph{i.e.}, $H_{T}>H_{S}$ and $W_{T}>W_{S}$), we first use average pooling to scale down the dimensions of the teacher network's feature maps to match the student network's scale:
\begin{equation}
\mathcal{P}^{T}_{\text{fuse}}=\text{AvgPool}(\mathcal{P}^{T}_{\text{fuse}}, (H_{S}, W_{S})).
\end{equation}
Meanwhile, if the feature map dimensions of the student network are larger than those of the teacher network, the features of the student network are also scaled as:
\begin{equation}
\mathcal{P}^{S}_{\text{fuse}}=\text{AvgPool}(\mathcal{P}^{S}_{\text{fuse}}, (H_{T}, W_{T})).
\end{equation}
Subsequently, the fused features $\mathcal{P}^{S}_{\text{fuse}}$ are projected to align the channel dimension of $\mathcal{P}^{T}_{\text{fuse}}$:
\begin{equation}
\mathcal{P}^{S}_{\text{fuse}} =  \delta(\mathbf{W}_{2}\delta(\mathbf{W}_{1}\mathcal{P}^{S}_{\text{fuse}})).
\end{equation}
Here, $\mathbf{W}_{1}\in \mathbb{R}^{\frac{C_{S}}{r}\times C_{S}}$, and $\mathbf{W}_{2}\in \mathbb{R}^{C_{T}\times  \frac{C_{S}}{r}}$ are the weights for two linear layers, respectively, and $\delta$ is the ReLU activation function. After dimension alignment, the fused features $\mathcal{P}^{T}_{\text{fuse}}$ and $\mathcal{P}^{S}_{\text{fuse}}$ can be subjected to subsequent feature activation operation and domain-invariant feature transfer operation.
\begin{table}[t]
	\centering
	\resizebox{\linewidth}{!}{
		\begin{tabular}{ccccc|c}
			\hline
			\#Conv & Kernel size  & \#Params & \#Params$^{A}$/\#Params$^{T}$& FLOPs & Avg   \\ \hline
			1      & 1$\times$1   &  1.05M  & 4.82\%   & 51.78M      & 82.09 \\ 
			2      & 1$\times$1   &  0.52M  & 2.38\%    & 26.19M      & \textbf{82.77} \\ 
			3      & 1$\times$1   &  0.60M  & 2.75\%   & 29.50M      & 82.57 \\ 
			4      & 1$\times$1   &  0.66M  & 3.03\%   & 32.81M      & 82.46 \\ 
			5      & 1$\times$1   &  0.73M  & 3.35\%   & 36.12M      & 82.48 \\ \hline
			1      & 3$\times$3   &  9.44M  & 43.30\%   & 462.82M     & 82.41 \\ 
			2      & 3$\times$3   &  4.72M  & 21.65\%   & 231.71M     & 82.35 \\ 
			3      & 3$\times$3   &  5.31M  & 24.35\%   & 260.71M     & 82.46 \\ 
			4      & 3$\times$3   &  5.90M  & 27.06\%   & 289.71M     & 82.43 \\ 
			5      & 3$\times$3   &  6.49M  & 29.77\%   & 318.71M      & 82.33 \\ \hline
	\end{tabular}}
	\caption{Average classification accuracies (\%) of the student networks trained by our method using adapters with different structures on the 12 tasks for the Office-Home dataset. ``\#Conv'', ``Kernel size'', ``\#Params'', and ``FLOPs'' denote the number of convolutional layers, the size of the convolutional kernel, the number of learnable parameters, and the FLOating-Point operations (FLOPs) in the related adapter, respectively. Meanwhile, ``\#Params$^{A}$/\#Params$^{T}$" denotes the ratio of adapter and teacher network parameters, and ``M" stands for million.}
	\label{table_adapter}
\end{table}
\subsection{Structure Analysis of Knowledge Adapter}
\label{sec:saka}
In this subsection, we analyze the effect of knowledge adapters with different structures. In our proposed 4Ds, we default to configure the adapter with two 1$\times$1 convolution layers followed by BN layers and ReLU activation function. Here, we conduct experiments with adapters composed of varying numbers of convolution layers with different sizes of convolutional kernel in the teacher network. We select the teacher-student pair ResNet34-ResNet18 to evaluate on the Office-Home dataset. Moreover, we input an image of size 3$\times$224$\times$224 into the teacher network to calculate the FLOating-Point operations (FLOPs) required for the adapters, which is widely used to estimate the computational costs.
 
Table~\ref{table_adapter} reports the experimental results. Firstly, we can find that the adapter with two 1$\times$1 convolution layers has the least number of parameters and computations while achieving the best performance. Therefore, we reasonably used this structure configuration of the knowledge adapter in our method. Secondly, although the adapters with 1$\times$1 convolutional layers have significantly fewer parameters and FLOPs than those with 3$\times$3 convolutional layers, their performance is comparable to that of the adapters with 3$\times$3 convolutional layers. This indicates that adapters with 1$\times$1 convolutional layers are sufficient to capture the domain-specific knowledge from the target domain. Note that adapters with only one convolutional layer have significantly higher parameters and FLOPs than adapters with multiple convolutional layers. This is because adapters with only one convolutional layer cannot utilize scaling parameters to reduce parameters and FLOPs.
\begin{figure}[t]
	\centering
	\includegraphics[scale=0.32]{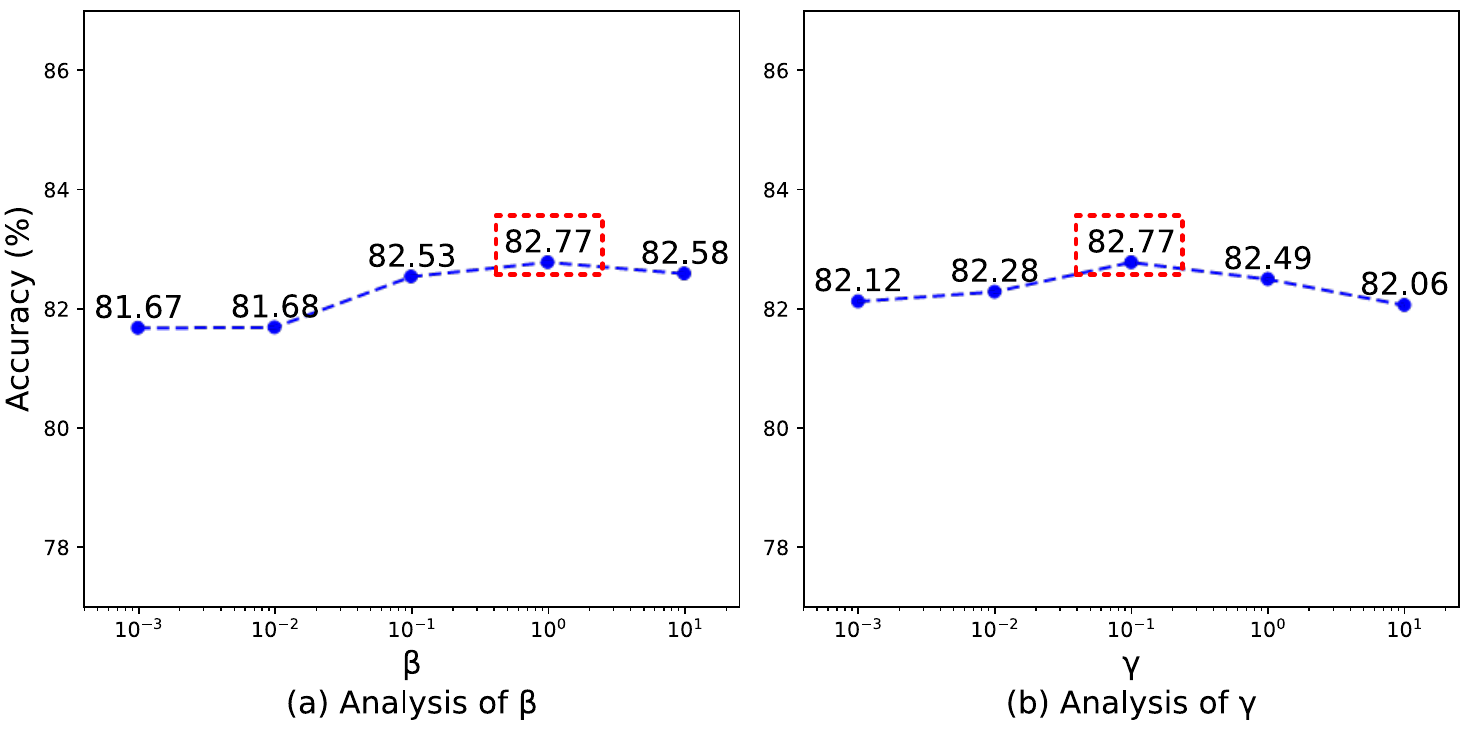}
	\caption{Parametric sensitivities of (a) $\beta$ and (b) $\gamma$ in Eq.~(\ref{eq_totals}).}
	\label{fig_ps}
\end{figure}
\subsection{Parametric Sensitivity}
\label{sec:ps}
In our proposed 4Ds, there are two tuning parameters $\beta$=1.0 and $\gamma$=0.1 in Eq.~\eqref{eq_totalt} and Eq.~\eqref{eq_totals}. Here, we analyze the sensitivity of our 4Ds to these parameters on the Office-Home dataset with the teacher-student pair ResNet34-ResNet18. We examine the average accuracies of twelve tasks in the Office-Home dataset by changing one parameter while maintaining the others.

Fig.~\ref{fig_ps} illustrates the test accuracy curve for the student network when parameters change. The parameters $\beta$ and $\gamma$ fluctuate within \{0.001, 0.01, 0.1, 1.0, 10\}. Despite these parameters varying across a broad scope, we can observe that the accuracy curve for the student network maintains general stability. These experimental results indicate that the performance of the student network is robust to parameter modifications. Consequently, the parameters in our 4Ds are readily adjustable.
\begin{figure*}[t]
	\centering
	\includegraphics[scale=0.52]{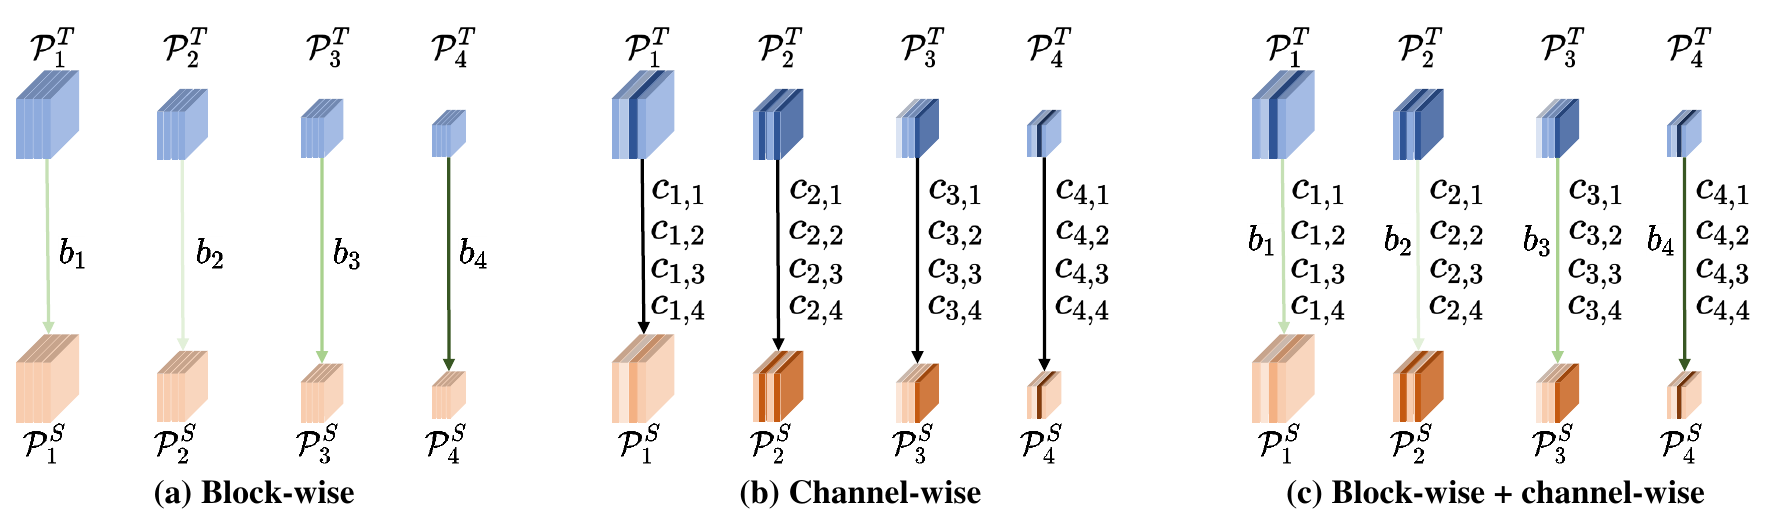}
	\caption{The diagram of various weighting strategies. (a) Block-wise weighting strategy assigns a weight to the features produced by each block. (b) Channel-wise weighting strategy distributes weight to each feature map within each block. (c) Block-wise + channel-wise weighting strategy assigns a weight to each block as well as to the feature maps within them. In this figure, ``$b$'' and ``$c$'' represent the weights for specific blocks and feature maps, respectively.}
	\label{fig_varweight}
\end{figure*}
\subsection{Weighting Strategy}
\label{sec:ws}
In ablation studies, we employ various weighting strategies to calculate the attention weights for the domain-invariant features of the teacher network and student network. Here, we assume that both the teacher network and student network consist of 4 convolutional blocks, with each block having 4 feature maps. As shown in Fig.~\ref{fig_varweight}, there are various domain-invariant feature weighting strategies, including:\\
\textbf{1) Block-wise} weighting strategy treats the features produced by each block as a whole and assigns a uniform attention weight to the features of each block. \\
\textbf{2) Channel-wise} weighting strategy considers each feature map in the feature block separately and assigns an independent weight to each feature map.\\
\textbf{3) Block-wise + channel-wise} weighting strategy assigns an attention weight to each feature block and the feature maps within it.\\
